# Supplementary material for: GRAP-MOT: Unsupervised Graph-based Position Weighted Person Multi-camera Multi-object Tracking in a Highly Congested Space
Source: arXiv:2510.21482 source file (2025-10-24)
Supplement: Supplementary file 1 [file SupplementaryFigures.pdf]

# Supplementary figures

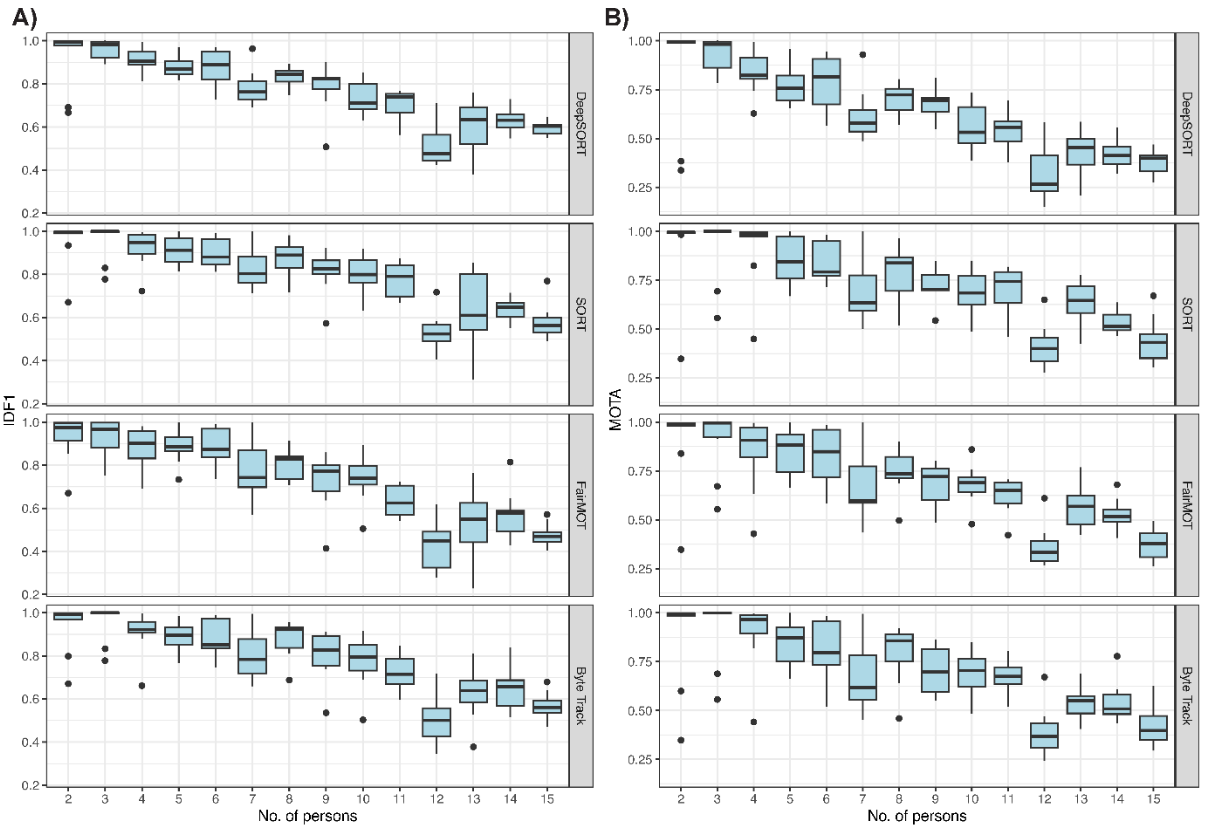


***Supp. Fig. 1.*** *Comparison of tracking methods' performance on the internal dataset in terms of IDF1 (A) and MOTA (B) indices. Recordings were grouped by the number of people present in the scene (x-axis).*

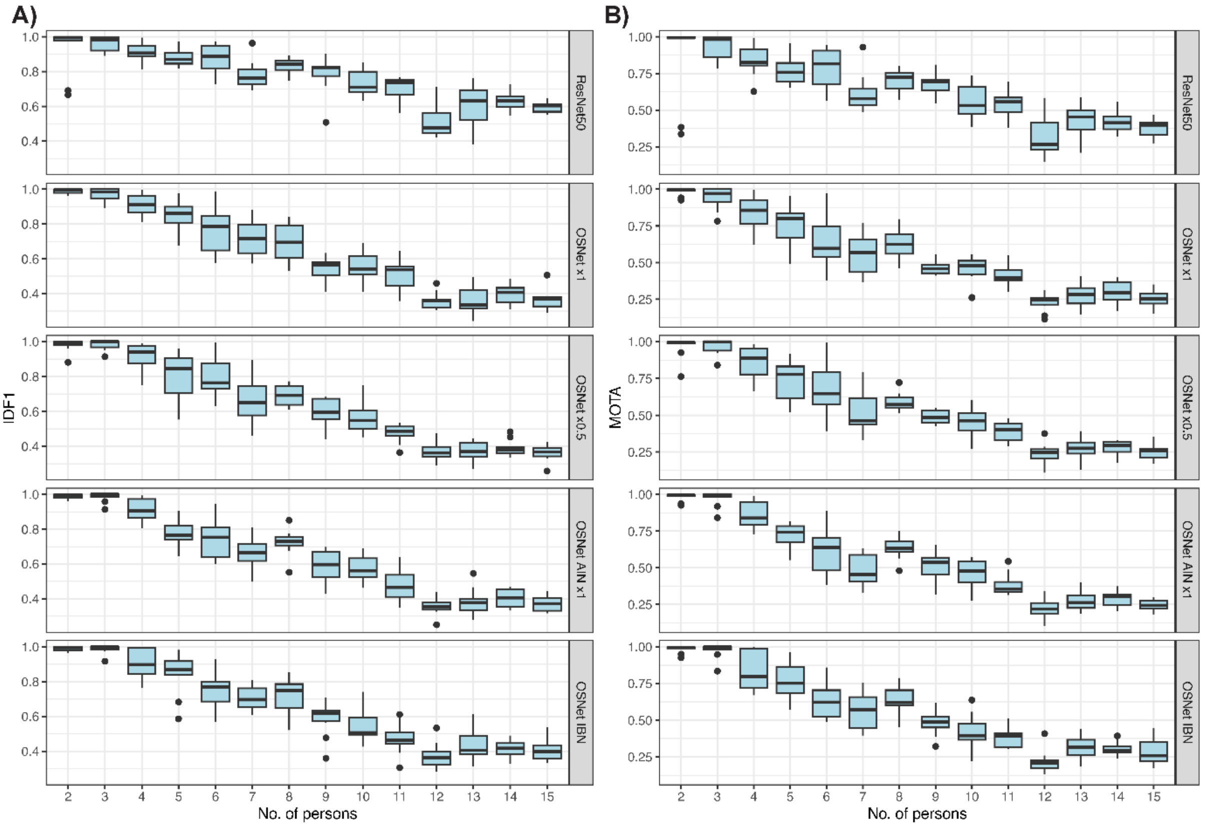


***Supp. Fig. 2****. Comparison of neural network models' performance on the internal dataset in terms of IDF1 (A) and MOTA (B) indices. Recordings were grouped by the number of people present in the scene (x-axis).*

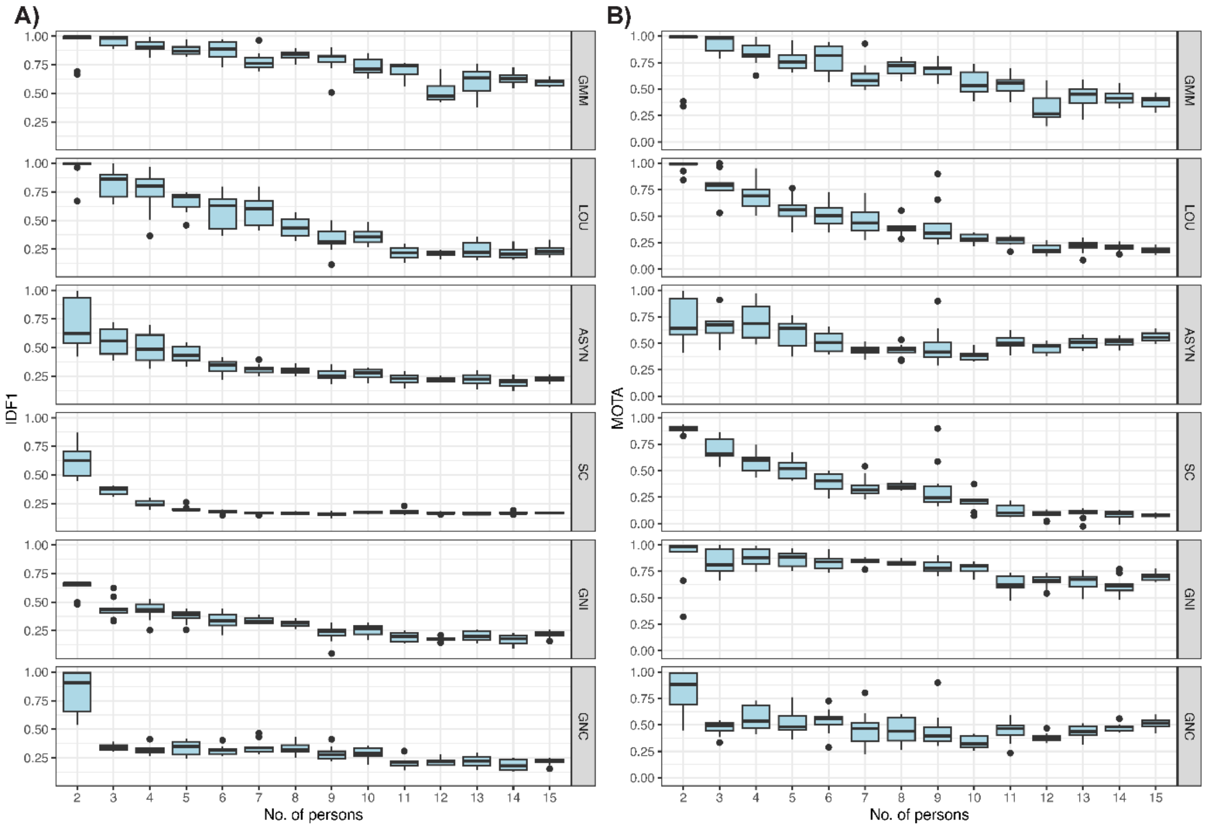


***Supp. Fig. 3.*** *Comparison of community detection algorithms' performance on the internal dataset in terms of IDF1 (A) and MOTA (B) indices. Recordings were grouped by the number of people present in the scene (x-axis).*

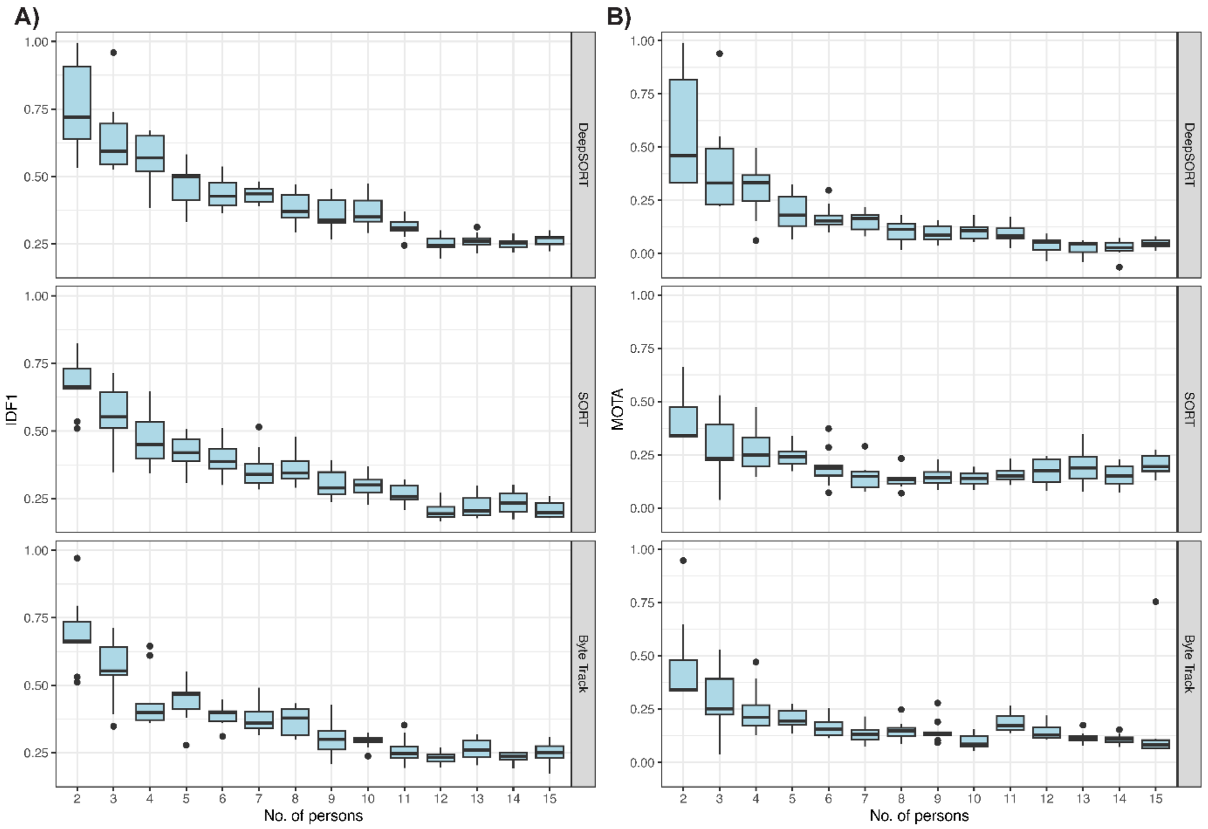


***Supp. Fig. 4.*** *Comparison of tracking methods' performance on the internal dataset in terms of IDF1 (A) and MOTA (B) indices without position estimation module. Recordings were grouped by the number of people present in the scene (x-axis).*

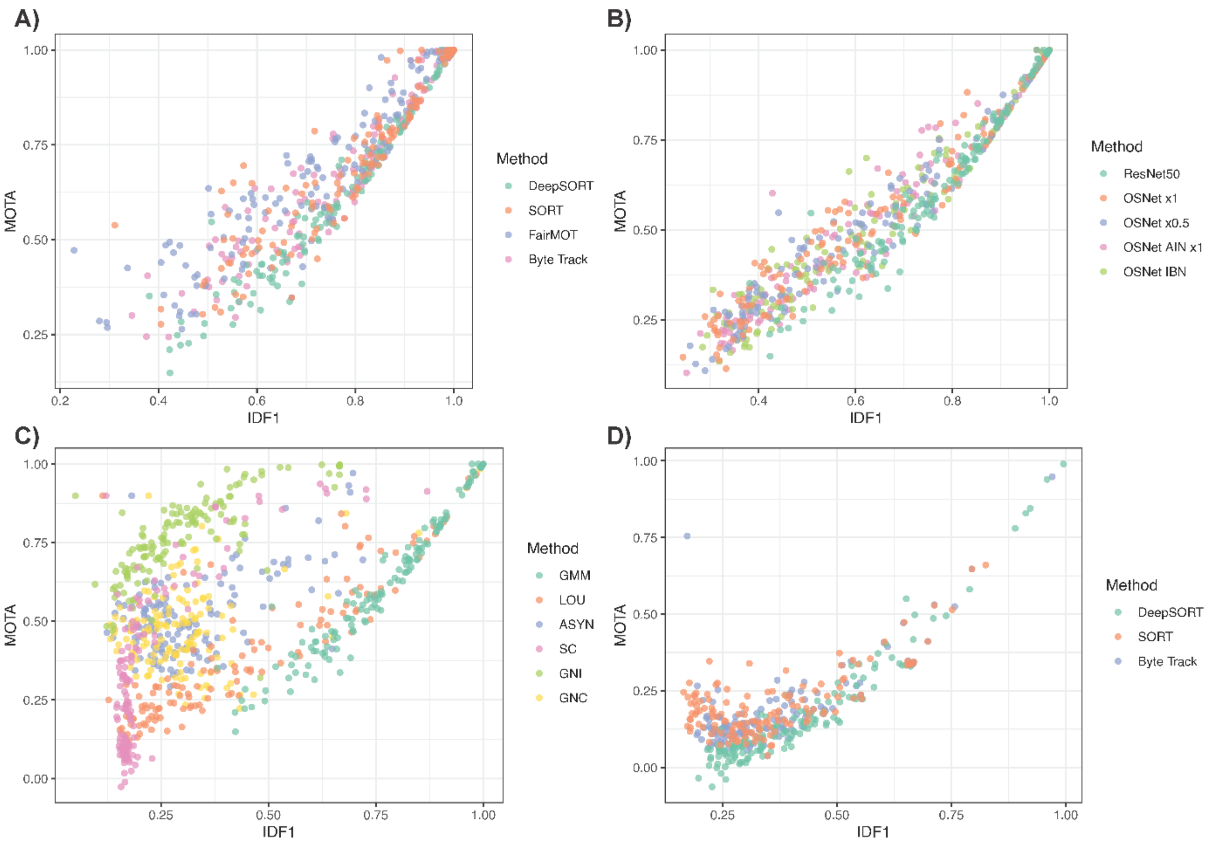


***Supp. Fig. 5****. Relationship between IDF1 and MOTA indices for the following testing scenarios: (A) tracking methods; (B) neural network models; (C) community detection algorithms; (D) tracking methods without position estimation module*
