# Supplementary material for: GRAP-MOT: Unsupervised Graph-based Position Weighted Person Multi-camera Multi-object Tracking in a Highly Congested Space
Source: arXiv:2510.21482 source file (2025-10-24)
Supplement: Supplementary file 2 [file SupplementaryTables.pdf]

TABLE I

TRACKING METHODS' PERFORMANCE COMPARISON ON THE INTERNAL DATASET. RECORDINGS WERE GROUPED BY THE NUMBER OF PEOPLE PRESENT IN THE SCENE AND THE MEDIAN OF THE CREATE GROUP METRICS IS SHOWN IN THE TABLE.

| task   | DeepSORT      |        | SORT           |         | FairMOT |        | Byte Track    |        |
|--------|---------------|--------|----------------|---------|---------|--------|---------------|--------|
|        | IDF1          | MOTA   | IDF1           | MOTA    | IDF1    | MOTA   | IDF1          | MOTA   |
| gt2    | 99.542        | 99.336 | <b>99.783</b>  | 99.708  | 97.513  | 98.851 | 99.207        | 99.493 |
| gt3    | 98.233        | 98.193 | <b>100.000</b> | 100.000 | 96.640  | 99.641 | 99.942        | 99.883 |
| gt4    | 90.579        | 82.363 | <b>94.864</b>  | 98.471  | 90.202  | 90.705 | 92.147        | 96.558 |
| gt5    | 86.968        | 75.759 | <b>91.218</b>  | 84.415  | 88.569  | 88.188 | 89.516        | 87.106 |
| gt6    | <b>88.859</b> | 81.589 | 88.077         | 79.256  | 87.375  | 84.917 | 85.148        | 79.569 |
| gt7    | 76.228        | 57.876 | <b>80.359</b>  | 63.546  | 74.299  | 59.935 | 78.378        | 61.852 |
| gt8    | 84.391        | 72.349 | 88.949         | 83.876  | 83.048  | 73.503 | <b>92.246</b> | 85.611 |
| gt9    | 82.330        | 69.502 | <b>82.625</b>  | 70.210  | 77.298  | 72.061 | 82.612        | 69.701 |
| gt10   | 71.057        | 53.178 | <b>79.965</b>  | 68.456  | 73.958  | 68.952 | 79.325        | 70.373 |
| gt11   | 73.854        | 55.682 | <b>79.097</b>  | 74.328  | 62.523  | 65.109 | 71.475        | 67.386 |
| gt12   | 47.630        | 26.599 | <b>52.369</b>  | 39.974  | 44.948  | 33.255 | 50.093        | 36.699 |
| gt13   | 63.389        | 45.302 | 61.019         | 64.601  | 55.027  | 56.932 | <b>63.894</b> | 55.077 |
| gt14   | 63.120        | 41.246 | 64.899         | 51.310  | 57.913  | 51.669 | <b>65.664</b> | 50.791 |
| gt15   | <b>60.329</b> | 39.859 | 56.431         | 43.151  | 46.982  | 37.816 | 56.067        | 39.691 |
| MEDIAN | 79.279        | 63.689 | <b>81.492</b>  | 72.269  | 75.799  | 70.506 | 80.969        | 70.037 |
| MEAN   | 77.608        | 64.202 | <b>79.975</b>  | 72.950  | 74.021  | 70.110 | 78.980        | 71.414 |
| STD    | 14.701        | 21.339 | 15.115         | 18.938  | 17.189  | 20.228 | 15.074        | 20.285 |

TABLE II

NEURAL NETWORK MODELS' PERFORMANCE COMPARISON ON THE INTERNAL DATASET. RECORDINGS WERE GROUPED BY THE NUMBER OF PEOPLE PRESENT IN THE SCENE AND THE MEDIAN OF THE CREATE GROUP METRICS IS SHOWN IN THE TABLE.

| task   | ResNet50      |        | OSNet x1      |        | OSNet x0.5    |        | OSNet AIN x1  |        | OSNet IBN     |        |
|--------|---------------|--------|---------------|--------|---------------|--------|---------------|--------|---------------|--------|
|        | IDF1          | MOTA   | IDF1          | MOTA   | IDF1          | MOTA   | IDF1          | MOTA   | IDF1          | MOTA   |
| gt2    | 99.542        | 99.336 | <b>99.660</b> | 99.457 | <b>99.660</b> | 99.457 | <b>99.660</b> | 99.457 | <b>99.660</b> | 99.457 |
| gt3    | 98.233        | 98.193 | 98.512        | 97.024 | <b>99.955</b> | 99.910 | <b>99.955</b> | 99.910 | <b>99.955</b> | 99.910 |
| gt4    | 90.579        | 82.363 | 90.989        | 85.667 | <b>94.174</b> | 88.913 | 90.488        | 83.880 | <b>89.825</b> | 79.687 |
| gt5    | <b>86.968</b> | 75.759 | 86.134        | 79.977 | 84.540        | 77.814 | 76.440        | 74.249 | 86.878        | 75.179 |
| gt6    | <b>88.859</b> | 81.589 | 78.509        | 59.654 | 76.347        | 64.645 | 75.344        | 63.674 | 76.975        | 62.274 |
| gt7    | <b>76.228</b> | 57.876 | 71.698        | 56.704 | 65.037        | 46.323 | 66.579        | 45.402 | 69.664        | 57.029 |
| gt8    | <b>84.391</b> | 72.349 | 69.508        | 62.425 | 69.209        | 57.282 | 72.981        | 63.362 | 74.974        | 62.046 |
| gt9    | <b>82.330</b> | 69.502 | 56.499        | 45.788 | 59.453        | 48.498 | 59.691        | 53.572 | 61.875        | 48.755 |
| gt10   | <b>71.057</b> | 53.178 | 54.207        | 48.071 | 54.847        | 46.380 | 56.132        | 47.783 | 50.587        | 39.565 |
| gt11   | <b>73.854</b> | 55.682 | 53.719        | 39.594 | 48.672        | 40.270 | 46.638        | 35.563 | 46.372        | 39.281 |
| gt12   | <b>47.630</b> | 26.599 | 36.162        | 24.423 | 36.196        | 24.708 | 35.559        | 21.905 | 36.303        | 20.939 |
| gt13   | <b>63.389</b> | 45.302 | 33.367        | 28.359 | 36.918        | 27.462 | 37.720        | 26.220 | 40.538        | 31.688 |
| gt14   | <b>63.120</b> | 41.246 | 40.723        | 29.500 | 38.005        | 29.574 | 40.587        | 30.366 | 41.697        | 29.478 |
| gt15   | <b>60.329</b> | 39.859 | 37.067        | 25.225 | 36.783        | 25.865 | 37.185        | 24.309 | 39.847        | 25.803 |
| MEDIAN | <b>79.279</b> | 63.689 | 63.004        | 52.388 | 62.245        | 47.439 | 63.135        | 50.678 | 65.769        | 52.892 |
| MEAN   | <b>77.608</b> | 64.202 | 64.768        | 55.848 | 64.271        | 55.507 | 63.926        | 54.975 | 65.368        | 55.078 |
| STD    | <b>14.701</b> | 21.339 | 22.696        | 25.253 | 22.895        | 25.827 | 22.015        | 25.828 | 22.269        | 25.140 |

TABLE III

COMMUNITY DETECTION ALGORITHMS' PERFORMANCE COMPARISON ON THE INTERNAL DATASET. RECORDINGS WERE GROUPED BY THE NUMBER OF PEOPLE PRESENT IN THE SCENE AND THE MEDIAN OF THE CREATE GROUP METRICS IS SHOWN IN THE TABLE.

| task   | GMM           |        | LOU           |        | ASYN   |              | SC     |        | GNI    |        | GNC    |        |
|--------|---------------|--------|---------------|--------|--------|--------------|--------|--------|--------|--------|--------|--------|
|        | IDF1          | MOTA   | IDF1          | MOTA   | IDF1   | MOTA         | IDF1   | MOTA   | IDF1   | MOTA   | IDF1   | MOTA   |
| gt2    | 99.542        | 99.336 | <b>99.729</b> | 99.457 | 62.461 | 64.054       | 62.674 | 90.258 | 66.507 | 98.114 | 90.510 | 88.424 |
| gt3    | <b>98.233</b> | 98.193 | 86.196        | 78.944 | 55.860 | 67.419       | 37.660 | 66.001 | 43.275 | 80.897 | 33.659 | 49.357 |
| gt4    | <b>90.579</b> | 82.363 | 79.936        | 69.155 | 48.683 | 68.574       | 23.820 | 60.170 | 43.274 | 88.030 | 31.314 | 53.622 |
| gt5    | <b>86.968</b> | 75.759 | 70.930        | 56.042 | 43.059 | 64.361       | 19.680 | 52.020 | 38.957 | 88.365 | 34.796 | 48.218 |
| gt6    | <b>88.859</b> | 81.589 | 62.888        | 50.357 | 34.856 | 50.661       | 18.096 | 40.414 | 33.775 | 84.061 | 31.787 | 55.848 |
| gt7    | <b>76.228</b> | 57.876 | 60.287        | 43.488 | 31.363 | 43.772       | 16.722 | 31.609 | 33.003 | 85.119 | 33.695 | 46.611 |
| gt8    | <b>84.391</b> | 72.349 | 43.286        | 38.604 | 29.496 | 44.030       | 16.320 | 34.469 | 31.641 | 81.918 | 31.833 | 44.007 |
| gt9    | <b>82.330</b> | 69.502 | 31.112        | 34.104 | 25.422 | 41.536       | 15.528 | 24.166 | 24.181 | 77.932 | 27.777 | 39.393 |
| gt10   | <b>71.057</b> | 53.178 | 35.623        | 28.352 | 27.824 | 38.742       | 17.351 | 21.600 | 27.003 | 80.031 | 28.812 | 32.141 |
| gt11   | <b>73.854</b> | 55.682 | 21.823        | 27.620 | 23.076 | 49.988       | 17.801 | 9.993  | 19.992 | 62.146 | 21.427 | 46.564 |
| gt12   | <b>47.630</b> | 26.599 | 21.573        | 17.684 | 22.219 | 47.284       | 16.667 | 9.665  | 18.037 | 66.201 | 22.029 | 37.486 |
| gt13   | <b>63.389</b> | 45.302 | 22.070        | 23.224 | 22.371 | 50.836       | 16.038 | 10.364 | 20.004 | 67.319 | 22.238 | 43.672 |
| gt14   | <b>63.120</b> | 41.246 | 20.687        | 19.837 | 20.210 | 51.511       | 16.661 | 9.248  | 17.966 | 60.998 | 17.895 | 48.137 |
| gt15   | <b>60.329</b> | 39.859 | 23.014        | 18.126 | 23.455 | 55.458       | 16.746 | 7.656  | 22.569 | 69.915 | 21.636 | 51.611 |
| MEDIAN | <b>79.279</b> | 63.689 | 39.454        | 36.354 | 28.660 | 50.749       | 17.048 | 27.888 | 29.322 | 80.464 | 30.063 | 47.374 |
| MEAN   | <b>77.608</b> | 64.202 | 48.511        | 43.214 | 33.597 | 52.730       | 22.269 | 33.402 | 31.442 | 77.932 | 32.101 | 48.935 |
| STD    | 14.701        | 21.339 | 26.641        | 24.089 | 13.141 | <b>9.491</b> | 12.490 | 24.677 | 12.951 | 10.647 | 17.067 | 12.549 |

TABLE IV

MOT RESULTS WITHOUT POSITION ESTIMATION MODULE; PERFORMANCE COMPARISON ON THE INTERNAL DATASET. RECORDINGS WERE GROUPED BY THE NUMBER OF PEOPLE PRESENT IN THE SCENE AND THE MEDIAN OF THE CREATE GROUP METRICS IS SHOWN IN THE TABLE.

| task   | DeepSORT |        | SORT   |        | Byte Track |        |
|--------|----------|--------|--------|--------|------------|--------|
|        | IDF1     | MOTA   | IDF1   | MOTA   | IDF1       | MOTA   |
| gt2    | 72.054   | 45.997 | 66.336 | 34.166 | 66.339     | 34.075 |
| gt3    | 59.391   | 33.207 | 55.290 | 23.326 | 55.290     | 25.132 |
| gt4    | 56.904   | 33.375 | 45.064 | 24.805 | 39.866     | 21.155 |
| gt5    | 49.845   | 18.024 | 41.953 | 24.227 | 46.769     | 19.423 |
| gt6    | 42.763   | 15.417 | 38.727 | 18.763 | 39.920     | 15.544 |
| gt7    | 43.605   | 16.551 | 33.954 | 14.898 | 35.975     | 13.232 |
| gt8    | 37.123   | 11.406 | 34.470 | 13.440 | 37.836     | 14.870 |
| gt9    | 33.730   | 8.624  | 28.937 | 14.274 | 30.006     | 13.362 |
| gt10   | 35.029   | 10.746 | 30.014 | 14.011 | 29.633     | 8.489  |
| gt11   | 30.923   | 8.342  | 25.735 | 15.072 | 24.750     | 17.233 |
| gt12   | 24.532   | 5.279  | 19.384 | 17.713 | 23.302     | 12.880 |
| gt13   | 26.141   | 4.551  | 20.503 | 18.921 | 26.081     | 11.106 |
| gt14   | 25.417   | 2.770  | 23.348 | 15.127 | 23.621     | 10.885 |
| gt15   | 27.446   | 4.647  | 19.696 | 19.489 | 25.094     | 8.275  |
| MEDIAN | 36.076   | 11.076 | 31.984 | 18.238 | 32.991     | 14.116 |
| MEAN   | 40.350   | 15.638 | 34.529 | 19.159 | 36.034     | 16.119 |
| STD    | 14.044   | 12.571 | 13.435 | 5.585  | 12.470     | 6.771  |
